# Supplementary material for: Computational investigation of multivalent binding of a ligand coated particle: Role of shape, size and ligand heterogeneity from a free energy landscape perspective
Source: arXiv:1710.09246 source file (2018-03-06)
Supplement: Supplementary file 1 [file SI-28Feb18.pdf]

# Supplementary Material for "Computational investigation of multivalent binding of a ligand coated particle: Role of shape, size and ligand heterogeneity from a free energy landscape perspective"

M. McKenzie, S. M. Ha, A. Rammohan, R. Radhakrishnan, & N. Ramakrishnan*

March 4, 2018

## Contents

**S1 Intermediate and weak binders** 3

**S2 Constructing models for the functionalized particle** 4
S2.1 Using the golden ratio to discretize a unit sphere . . . . . . . . . . . . . . . . . . . . . . . 4
S2.2 Stereographic projection of the unit sphere . . . . . . . . . . . . . . . . . . . . . . . . . 5
S2.3 Constrained Monte Carlo relaxation of the ellipsoidal particle surface . . . . . . . . . . 5
S2.4 Construction of the surface normal and placement of ligands . . . . . . . . . . . . . . . 5

**S3 Particle dimensions as a function of particle aspect ratio** 6

**S4 Hybrid molecular dynamics and Monte Carlo scheme to evolve particle orientations** 7

**S5 Computing the NC rotational volume** 8

**S6 Effect of particle anisotropy on NC binding** 9

**S7 Configurational entropies as a function of ligand heterogeneity** 10

**S8 Effect of particle size for $\mathcal{K}_b^{\text{eff}} = 1.0$ N/m** 11

**S9 Multivalency distribution as a function of particle size** 12

**S10 Interactive data for an umbrella sampling trajectory** 13

## S1 Intermediate and weak binders

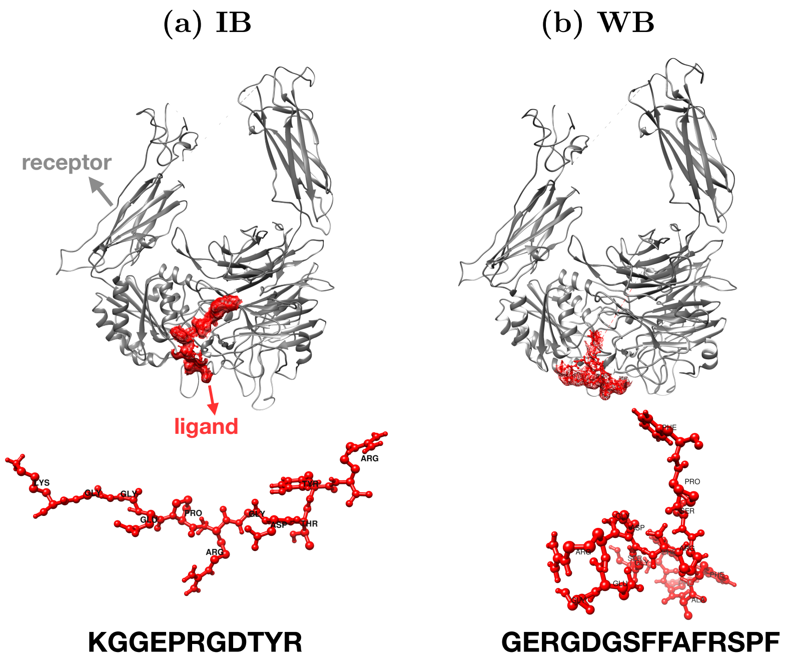


Figure S1: The top panels in (a) and (b) show snapshots of the IB and WB systems in their bound state– the receptor is shown in gray while the ligand is shown in red. The molecular structure of the peptide sequences KGGEPRGDTYR and GERGDGSFFAFRSPF that are the ligands for IB and WB systems, respectively, are displayed in the lower panels.

## S2 Constructing models for the functionalized particle

In this section, we describe the methods used to construct a functionalized particle with the required dimensions ($a$, $b$ and $c$), aspect ratio($\varepsilon$) and number of ligands ($N_l$). Model construction is done in four steps:

1. Discretization of the surface of a unit sphere into $N_l$ equally spaced vertices.
2. Stereographic projection of the unit sphere to the required dimensions.
3. Constrained Monte Carlo relaxation of the surface vertices
4. Construction of surface normal and placement of ligands.

The details of each of these methods are described below.

### *S2.1 Using the golden ratio to discretize a unit sphere*

Discretization of a sphere into $N_l$ equally spaced points is commonly done by starting from any of the five Platonic solids namely, the tetrahedron, cube, octahedron, dodecahedron and icosahedron. This method is not generic since it only works for very specific values of $N_l$. In our approach, we use a more generic method based on the golden angle:

$$\Phi_G = \pi \times (3 - \sqrt{5}). \tag{S1}$$

For a given value of $N_l$, we compute $z_i$, the $z$ position of the $i$ th vertex as:

$$z_i = \left(1 - \frac{1}{N_l}\right) - \frac{2}{N_l} \times (i - 1), \tag{S2}$$

and $\theta_i$ the polar angle for the $i$ th vertex as:

$$\theta_i = i\Phi_G. \tag{S3}$$

These in turn yield the $x$ and $y$ positions of the $i$ th vertex as:

$$x_i = \sqrt{1 - z_i{}^2}\cos\theta_i, \tag{S4}$$

and

$$y_i = \sqrt{1 - z_i{}^2}\sin\theta_i. \tag{S5}$$

A python based pseudo-code for the implementation of points on a sphere is provided in Listing 1.

```
## Generates a unit sphere with specified number of vertices such that
## all set of neighbouring points are equispaced.
from random import random,randint
import numpy,sys
n = Nl
golden_angle = numpy.pi * (3 - numpy.sqrt(5))
theta = golden_angle * numpy.arange(n)
z = numpy.linspace(1 - 1.0 / n, 1.0 / n - 1, n)
radius = numpy.sqrt(1 - z * z)
points = numpy.zeros((n, 3))
points[:,0] = radius * numpy.cos(theta)
```

```python
points[:,1] = radius * numpy.sin(theta)
points[:,2] = z
filename='N-'+str(n)+'-sphere.dat'
numpy.savetxt(filename,points,delimiter='\t')
```

Listing 1: A python implementation of the golden angle based method

### *S2.2 Stereographic projection of the unit sphere*

A spheroidal particle of the desired dimensions and aspect ratio is constructed by a stereographic projection of the vertex positions. If the unit sphere is centered at $(0, 0, 0)$ then the position of the $i$ th vertex of the spheroidal particle is computed as:

$$\begin{aligned} x_i &= ax_i, \\ y_i &= by_i, \\ z_i &= cz_i. \end{aligned} \tag{S6}$$

### *S2.3 Constrained Monte Carlo relaxation of the ellipsoidal particle surface*

The uniform spacing between the vertices is not preserved when the sphere is stereographically projected to a spheroid with aspect ratio $\varepsilon \neq 1$. To ensure that the vertices on a spheroid are equally spaced we employ a constrained Monte Carlo relaxation of the vertex position on the surface of the spheroid. In our approach, we model the interaction of a vertex with all other vertices as a purely repulsive potential $\mathcal{W}$, taken to be the Weeks-Chandler-Anderson (WCA) potential. Each Monte Carlo step is constituted of $N_l$ attempts to displace a randomly chosen vertex $i$ from its current position $(x_i, y_i, z_i)$ to a new position $(x_i + \delta x_i, y_i + \delta y_i, z_i + \delta z_i)$, such that the latter satisfies the constraint $((x_i + \delta x_i)/a)^2 + ((y_i + \delta y_i)/b)^2 + ((z_i + \delta z_i)/c)^2 = 1$. Each of the attempted moves is accepted using the Metropolis criterion with a probability $P_{\text{acc}} = \min(1.0, \exp(-\beta\Delta\mathcal{W}))$ – here $\Delta\mathcal{W}$ is the change in the repulsive potential due to the displacement of the vertex. The Monte Carlo runs were performed until the distance between all neigboring vertices converged to the same value.

### *S2.4 Construction of the surface normal and placement of ligands*

In our model for the functionalized particle, we take the ligands on the particle surface to be oriented along the radially outward direction, which coincides with the surface normal $\hat{n}$. While the base position of the $i$ th ligand is taken to be $(x_i^b, y_i^b, z_i^b) = (x_i, y_i, z_i)$, i.e., the same as the position of the $i$ th vertex, its tip position is computed as:

$$(x_i^t, y_i^t, z_i^t) = (x_i^b + L_l(\hat{n}_i \cdot \hat{x}), y_i^b + L_l(\hat{n}_i \cdot \hat{y}), z_i^b + L_l(\hat{n}_i \cdot \hat{z})). \tag{S7}$$

Here $L_l$ is the length of the ligand molecule and $\hat{n}_i$ is the outward pointing normal at the $i$ th vertex computed as:

$$\hat{n}_i = \left(\frac{\partial}{\partial x}, \frac{\partial}{\partial y}, \frac{\partial}{\partial z}\right)\left(\left(\frac{x_i^b}{a}\right)^2 + \left(\frac{y_i^b}{b}\right)^2 + \left(\frac{z_i^b}{c}\right)^2 - 1\right) = \left(\frac{2x_i^b}{a^2}, \frac{2y_i^b}{b^2}, \frac{2z_i^b}{c^2}\right). \tag{S8}$$

## S3 Particle dimensions as a function of particle aspect ratio

The dimensions of the ellipsoidal particles presented in Fig.7 of the main manuscript are shown in Table 1. Here we take all particles to have an equivalent volume, equal to that for a spherical particle of radius $50$ nm. The corresponding snapshots of the particles bound to the substrate are displayed in Fig. S2.

| | $\varepsilon = 0.1$ | $\varepsilon = 0.2$ | $\varepsilon = 0.5$ | $\varepsilon = 1.0$ | $\varepsilon = 2.0$ | $\varepsilon = 5.0$ | $\varepsilon = 10.0$ |
|---|---|---|---|---|---|---|---|
| $a$ (nm) | 107.7 | 85.5 | 63.0 | 50.0 | 39.7 | 29.2 | 23.2 |
| $b$ (nm) | 10.8 | 17.1 | 31.5 | 50.0 | 39.7 | 29.2 | 23.2 |
| $c$ (nm) | 107.7 | 85.5 | 63.0 | 50.0 | 79.4 | 146.2 | 232.1 |

Table 1: The dimensions $a$, $b$ and $c$ for particles with seven different aspect ratios in the range $\varepsilon = 0.1$–$10.0$.

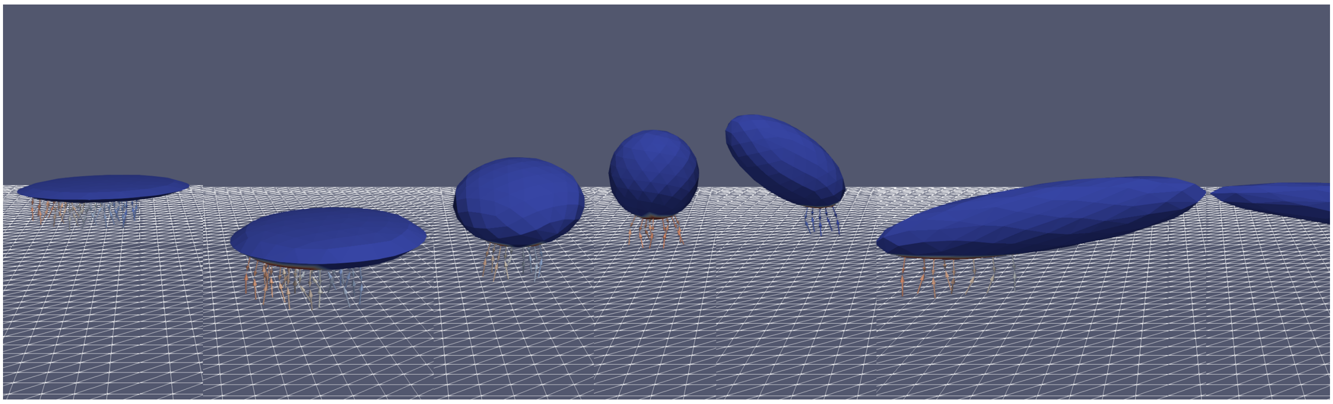

Figure S2: Ellipsoidal particles of different aspect ratio. The aspect ratio, $\epsilon$. From left to right, the value of $\epsilon$ corresponds to 0.1, 0.2, 0.5, 1.0, 2.0, 5.0, and 10.0, as noted in table 1.

## S4 Hybrid molecular dynamics and Monte Carlo scheme to evolve particle orientations

We evolve the rotational degrees of freedom of a spherical particle in terms of its Euler angles, as described in the methods section of the main manuscript. However, the use of Euler angles for anisotropic spheroidal particles will lead to singularities (also known as the gimbal lock) that can affect the rotational ergodicity of the particle [1]. Hence, we describe the rotational degrees of freedom for anisotropic particles in terms of their Cayley-Klein parameters, also called the Quaternions [1]. The particle orientation is described in terms of a four dimensional vector $(q_0, q_1, q_2, q_3)$ such that they satisfy (i) $-1 < q_n < 1$, for $n = 0, 1, 2, 3$, and (ii) $\sum_{n=0}^{3} q_n^2 = 1$.

One of the major difficulties in using Quaternions for Monte Carlo simulations lies in generating a distribution for $q_0$, $q_1$, $q_2$ and $q_3$ that samples the rotational space with a uniform density. Several schemes for generating this distribution have been proposed, for example see [2], but all of these methods show insufficient sampling when the particle is in a bound state. To alleviate the effect of sampling we resort to a molecular dynamics based technique to generate new values for the quaternions. This follows directly from the equations of motion for the quaternions given by [1]:

$$\begin{pmatrix} \dot{q}_0 \\ \dot{q}_1 \\ \dot{q}_2 \\ \dot{q}_3 \end{pmatrix} = \frac{1}{2} \begin{pmatrix} q_0 & -q_1 & -q_2 & -q_3 \\ q_1 & q_0 & -q_3 & q_2 \\ q_2 & q_3 & q_0 & -q_1 \\ q_3 & q_2 & q_1 & q_0 \end{pmatrix} \begin{pmatrix} 0 \\ \omega_x \\ \omega_y \\ \omega_z \end{pmatrix}. \tag{S9}$$

Here $\omega_x$, $\omega_y$ and $\omega_z$ are the angular velocities of the particle in the Cartesian frame. We use Eqn. (S9) to generate a random orientation by drawing the values of $\omega_x$, $\omega_y$ and $\omega_z$ from a normal distribution with zero mean and respective variances $\sigma_x^2$, $\sigma_y^2$ and $\sigma_z^2$. Here $\sigma_n^2 = (k_B T)/I_{nn}$ and $I_{nn}$ is the moment of inertia for rotation about the $n$ axis. The new orientation of the particle is obtained by integrating Eqn. (S9) which yields:

$$\begin{aligned} q_0(t+\Delta t) &= q_0(t) - (q_1(t)\omega_x - q_2(t)\omega_y - q_3(t)\omega_z)\,\Delta t, \\ q_1(t+\Delta t) &= q_1(t) + (q_0(t)\omega_x - q_3(t)\omega_y + q_2(t)\omega_z)\,\Delta t, \\ q_2(t+\Delta t) &= q_2(t) + (q_3(t)\omega_x + q_0(t)\omega_y - q_1(t)\omega_z)\,\Delta t, \\ q_3(t+\Delta t) &= q_3(t) + (q_2(t)\omega_x + q_1(t)\omega_y + q_0(t)\omega_z)\,\Delta t. \end{aligned} \tag{S10}$$

Here $t$ denotes an arbitrary time point and $\Delta t$ is the timestep for integration. The new orientation of the particle is then accepted based on canonical Monte Carlo using the Metropolis scheme with a probability $P_{\text{acc}} = \min(1, \exp(-\beta\Delta\mathcal{H}))$. The value of $\Delta t$ is adjsuted during runtime so that nearly $50\%$ of the attempted moves are accepted. This hybrid scheme provides an efficient technique to simulate the fluctuations in the quaternions and hence the rotational motion of anisotropic objects.

## S5 Computing the NC rotational volume

The fluctuations in the NC Euler angles yield useful information about the T3 term described in Eqn. (9) of the main manuscript. The three Euler angles $(\phi, \theta, \psi)$ can either show a flat or normal distribution depending upon the degree of binding of the NC. These two cases are shown in Figs. S3(a) and (b), respectively, where the best fit curves for each distribution are shown as thick solid lines.

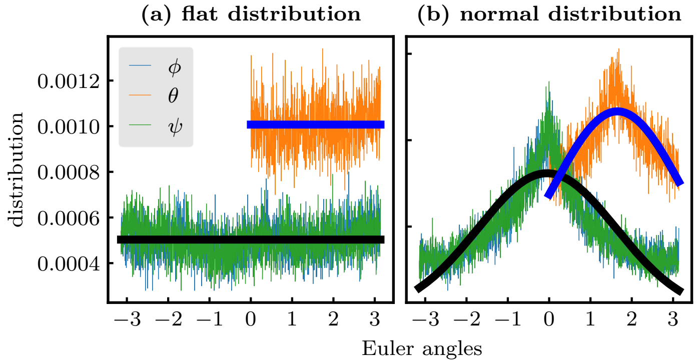


Figure S3: The two types of Euler angle distributions seen in our simulations. Panel (a) shows a flat distribution for all three Euler angles $\phi$, $\theta$ and $\psi$, while panel (b) shows a normal distribution for all three angles.

The flat distribution is normally seen when the NC is either in an unbound state or when $d^*$, the cutoff distance for binding, is very large, while the normal distribution are observed for all other cases. Following Carlsson and Aqvist [3], we compute the rotational volume for a NC with normal distribution of Euler angles as:

$$\text{rotational volume} = \sigma_{\phi_p}\sigma_{\cos\theta_p}\sigma_{\psi_p} \tag{S11}$$

where $\sigma$ denotes the standard deviation. It should be noted that the standard deviation for $\theta_p$ is computed over its cosine value. On the other hand, for NCs showing a flat distribution, as in Fig. S3(a), we take the rotational volume to be:

$$\text{rotational volume} = 8\pi^2. \tag{S12}$$

## S6 Effect of particle anisotropy on NC binding

Here we display the effect of particle shape on the multivalency profile for the IB and SB systems, with $\mathcal{K}_b^{\text{eff}} = 1.0$ N/m. The corresponding data are shown in Figs. S4 and S5, respectively. For the IB system, there is no considerable change in the multivalency distribution since $P(m = 0) \sim 1.0$ for all values of the aspect ratio studied here. The SB on the other hand, shows a high sensitivity with decrease in particle aspect ratio (for example compare $P(m)$ for $\varepsilon = 1.0$ to that for $\varepsilon = 0.1$ in Fig. S5) while there is no noticeable change in $P(m)$ as the aspect ratio increases.

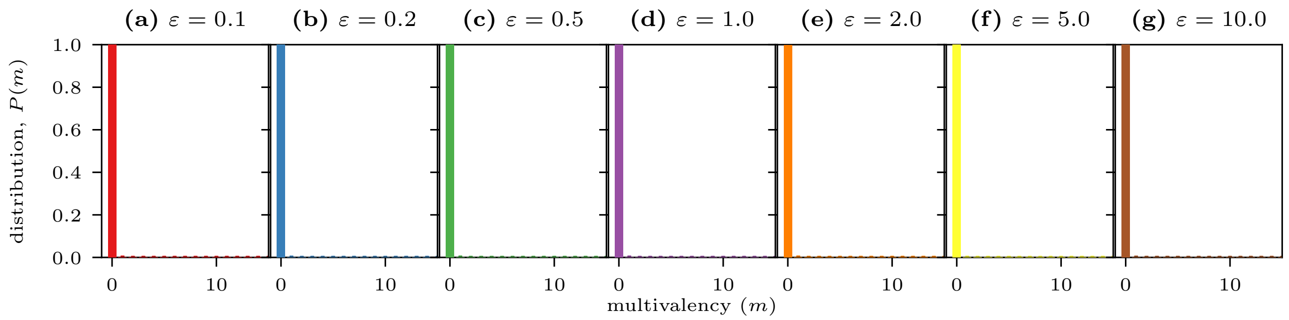


Figure S4: Multivalency distribution for spheroidal particles with $\varepsilon = 0.1, 0.2, 0.5, 1.0, 2.0, 5.0$ and $10.0$ for the IB system with $\mathcal{K}_b^{\text{eff}} = 1.0$ N/m. All particles were taken to bind to a substrate with 2000 receptors/$\mu$m$^2$.

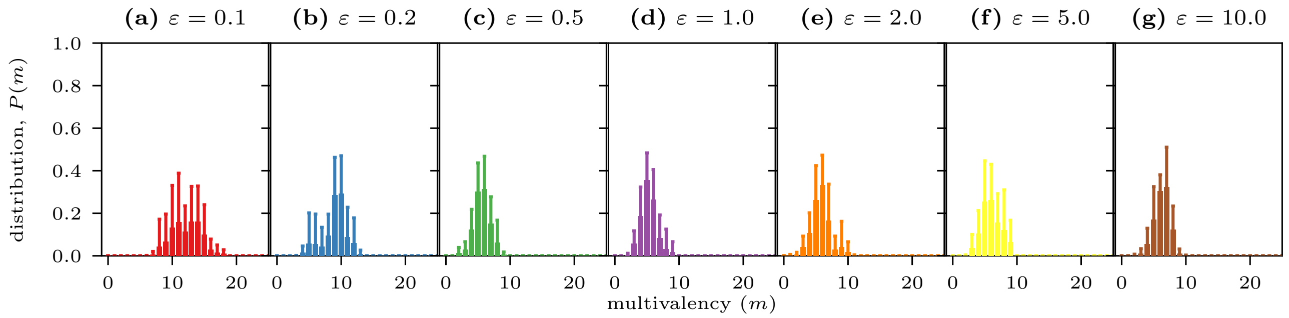


Figure S5: Multivalency distribution for spheroidal particles with $\varepsilon = 0.1, 0.2, 0.5, 1.0, 2.0, 5.0$ and $10.0$ for the SB system with $\mathcal{K}_b^{\text{eff}} = 1.0$ N/m. All particles were taken to bind to a substrate with 2000 receptors/$\mu$m$^2$.

## S7 Configurational entropies as a function of ligand heterogeneity

Changes in the ligand concentration has a minimal effect on T1, T2 and T3 terms. This is shown in Fig. S6 for a 50 nm spherical NC with varying compositions of SB:IB ligands. The data in panels (d) and (e) are the same as shown in Fig.8 of the main manuscript.

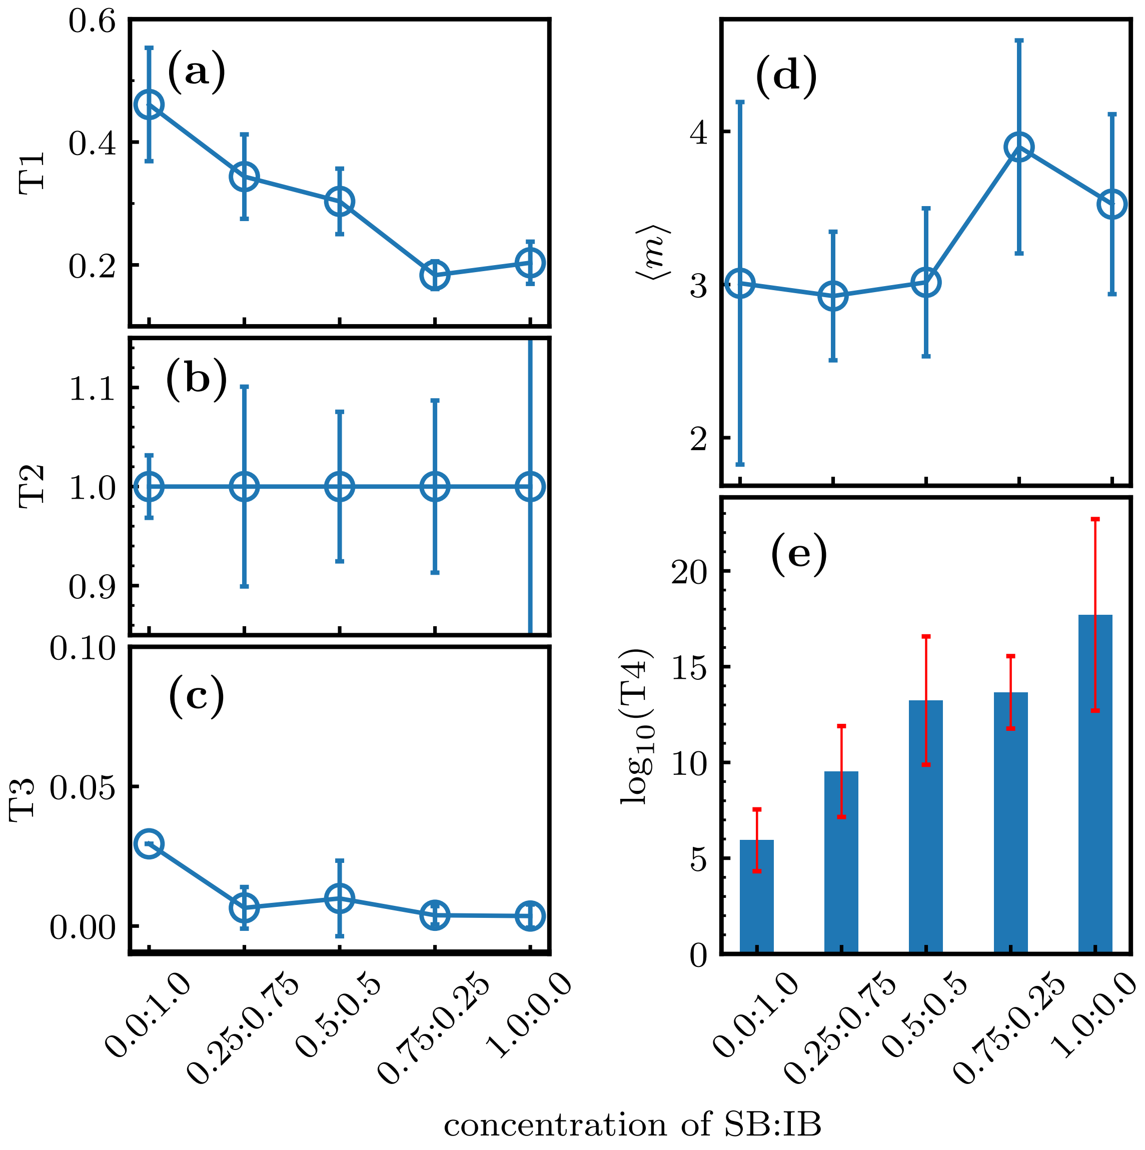


Figure S6: The T1, T2 and T3 terms as a function of SB:IB ligand composition are shown in panels (a), (b) and (c), respectively. The average multivalency at equilibrium $\langle m \rangle$ and the T4 term are shown in panel (d) and (e).

## S8 Effect of particle size for $\mathcal{K}_b^{\mathrm{eff}} = 1.0$ N/m

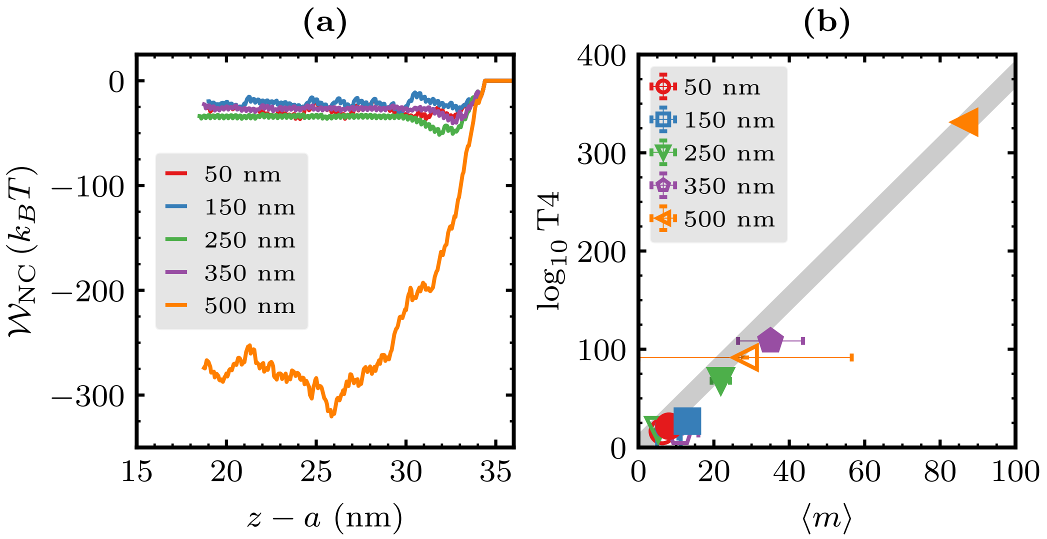


Figure S7: (a) The potential of mean force $\mathcal{W}_{\mathrm{NC}}$ is shown for five different particle sizes functionalized with the SB ligand with $\mathcal{K}_b^{\mathrm{eff}} = 1.0$ N/m. (b) The correlation between T4 and $\langle m \rangle$ as described in Fig.9 of the main manuscript.

## S9 Multivalency distribution as a function of particle size

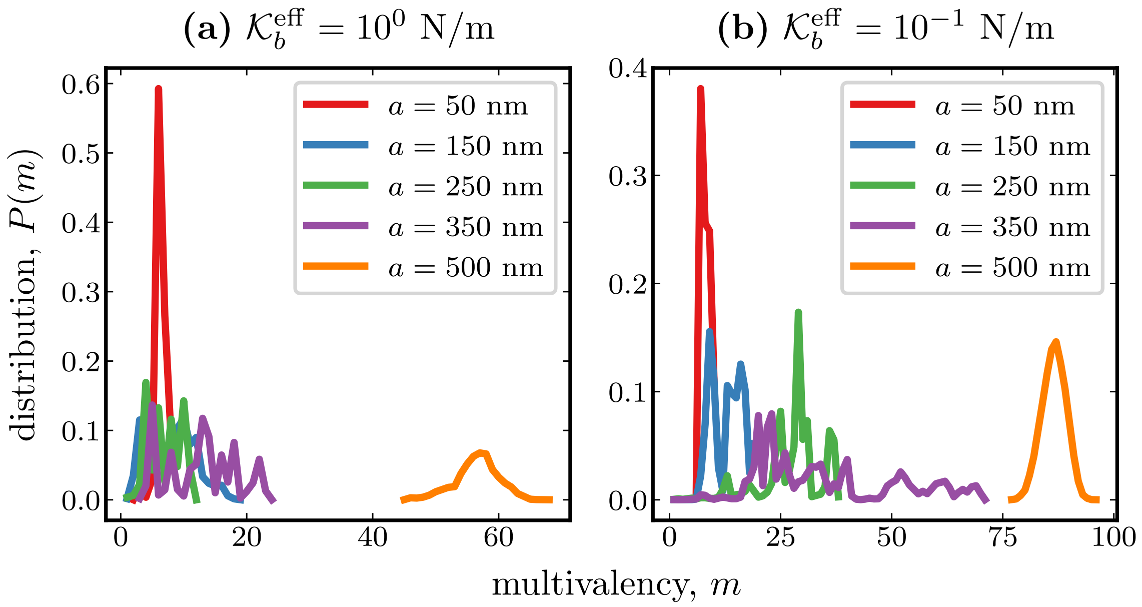


Figure S8: $P(m)$, the multivalent distribution as a function of particle size for $\mathcal{K}_b^{\rm eff} = 1.0$ N/m (a) and $\mathcal{K}_b^{\rm eff} = 0.1$ N/m (b). For both systems, particles with size $a = 50$ nm and $500$ nm show unimodal distributions in the multivalency $m$, while particles with sizes in the range $150$–$350$ nm show multimodal multivalency distributions.

## S10 Interactive data for an umbrella sampling trajectory

We have provided an interactive HTML file that shows six different measures along an umbrella sampling trajectory with 120 windows. A snapshot of the interactive panel is displayed in Fig. S9. These measures are shown in Fig. 4 of the main manuscript and also in Fig. S3. The data corresponds to a spherical NC with $a = b = c = 50$ nm, with SB receptor-ligands and $\mathcal{K}_b^{\text{eff}} = 0.1$ N/m. The position of the umbrella sampling window can be changed by moving the slider on the top left in Fig. S9. The position of the window $Z_{P,0}$ is shown alongside and is also given by the position of the red dot in the top right panel.

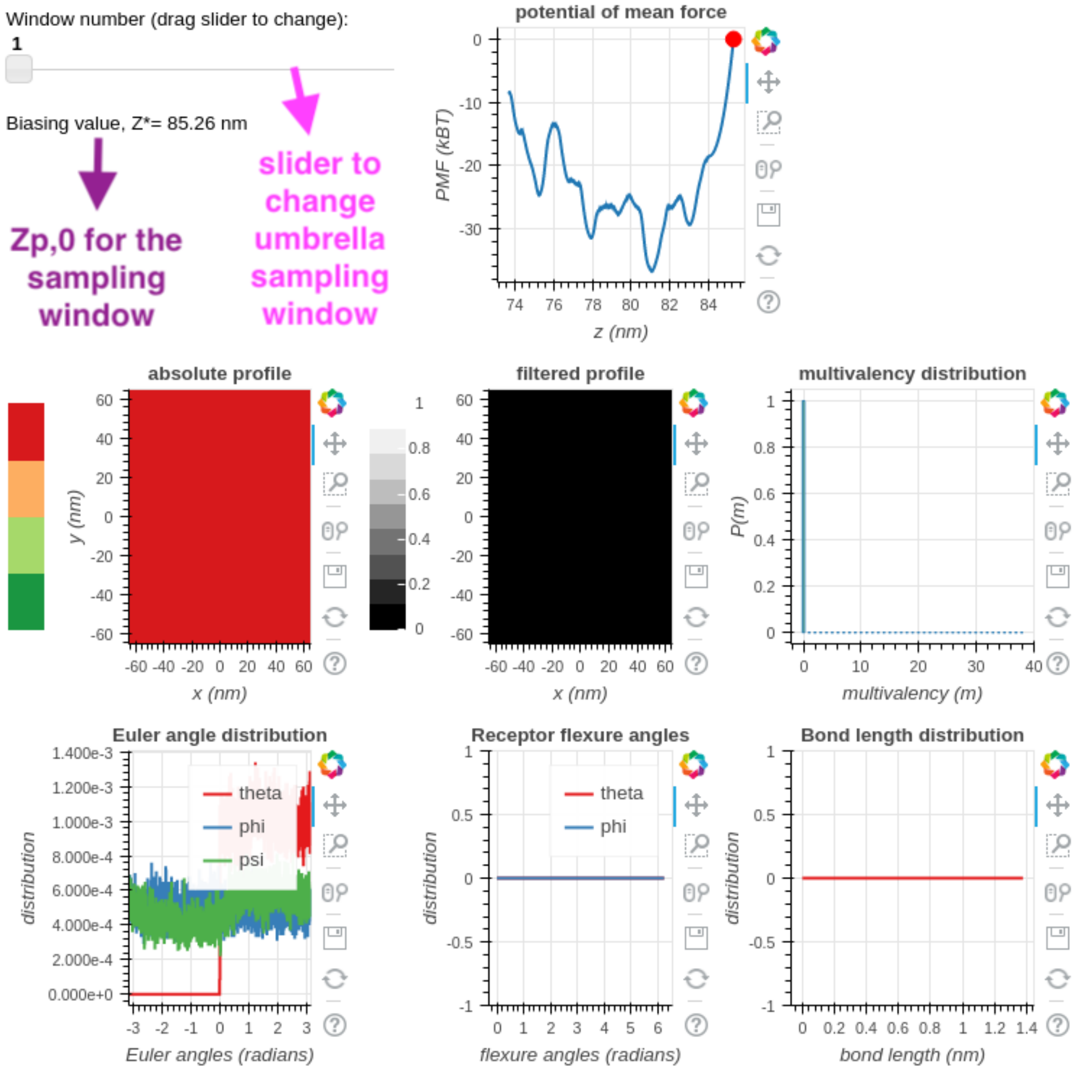


Figure S9: A snapshot of the interactive panel that shows (i) PMF (top right), (ii) localization profile of bound receptor (middle left and center), (iii) multivalency distribution (middle right), (iv) Euler angle distribution (bottom left), (v) receptor flexure distribution (bottom center), and (vi) bond length distribution (bottom right) for an umbrella sampling trajectory of a 50 nm spherical particle, coated with SB ligands that interact with $\mathcal{K}_b^{\text{eff}} = 0.1$ N/m.

## Supporting References


[1] Allen, M. P., and D. J. Tildesley, 1989. Computer Simulation of Liquids (Oxford Science Publications). Oxford science publications. Oxford University Press, reprint edition.

[2] Kuffner, J. J., 2004. Effective sampling and distance metrics for 3D rigid body path planning. In IEEE International Conference on Robotics and Automation, 2004. Proceedings. ICRA '04. 2004. IEEE, 3993–3998.

[3] Carlsson, J., and J. Aqvist, 2005. Absolute and Relative Entropies from Computer Simulation with Applications to Ligand Binding. J. Phys. Chem. B 109:6448–6456.
